# Supplementary material for: PARI: A Probabilistic Approach to AS Relationships Inference
Source: arXiv:1905.02386 source file (2019-05-07)
Supplement: Supplementary file 1 [file appendix.tex]

\section{Appendix}
\subsection{Content Wait List}
\subsubsection{Future Works}
\todo{[Might be put to the end of \S\ref{sec:conclusion} if it fits]} One of the directions for future work is to examine how well~\acrshort{pari} is able to capture uncertainty in an evolving Internet topology. For example, we look forward to acquiring the latest snapshot of validation dataset to determine whether the probabilistic model learned from an older snapshot remains applicable. Another direction is to extend our paradigm and effectively incorporate multiple assumptions and heuristics that might lead to different outputs when applied individually. Finally, we believe it is a promising direction to explore scalable approaches to expressing uncertainty in both the rules applied and the inference outputs generated.
%Our paradigm allows future works to further exploit ``negative observations'', or the set of observations that are not available 

\subsubsection{Complex AS Relationships}
\label{sec:complex-rel}
\todo{[Might be put to the end of \S\ref{sec:uncertainty} if it fits]} The existence of complex AS relationships implies that classifying certain links into one of the three traditional types of relationships (c2p, p2p, s2s) can be less precise and over-simplified.~\cite{giotsas2014inferring} identified two complex types: (1) the hybrid relationship where the type of relationship varies depending on the interconnection points; and (2) the partial transit relationship where an AS transits traffic from another AS to its peers and customers but not providers. The concept of hybrid relationship represents a source of uncertainty because it challenges most algorithms' fundamental assumption that each link is associated with a single type of relationship and without additional information there is no known strategy to determine whether a relationship is hybrid or not. Furthermore, it highlights the need to revisit rules, such as the valley-free constraint, that underline these algorithms as they might not be applicable to hybrid relationship inference.

%While the estimated number of links with hybrid relationhips is low~\cite{giotsas2014inferring}, we can no longer apply the valley-free constraint in a naive manner.

In this paper we limit ourselves to the traditional types of relationships and it is part of our future work to extend our analysis into complex AS relationships.

\subsubsection{Effect of Relaxation}
\todo{[This part can go into \S\ref{sec:evaluation}.]} Prior to the relaxation step to dismantle unsatisfiable components, \acrshort{pari} generates a total of 38,009 connected components at line~\ref{lst:line:components} of Algorithm~\ref{algo:comp-sv}. 37,668 of them contains a single node, which means that the inference of the corresponding AS link does affect or depend on other AS links. We refer to them as \textit{trivial} components because their score vectors can be determined by examining the valley-free constraints imposed on the single AS link. We note that 606 trivial components are unsatisfiable. It means it is impossible to make inference for AS links covered by these components without violating the valley-free constraint. Accordingly, the remaining 341 components are \textit{non-trivial} and \acrshort{pari} must respect the interdependence across multiple AS links. The blue curve in Figure~\ref{fig:cc-cdf} plots the size distribution of non-trivial connected components. The majority have fewer than 100 nodes. But the largest component contains over 8000 nodes. It is also one of the 8 unsatisfiable non-trivial components. The non-trivial components cover approximately 25\% of the AS links in the step of probabilistic inference.

\begin{figure}[!htb]
	\centering
	\includegraphics[width=0.4\paperwidth]{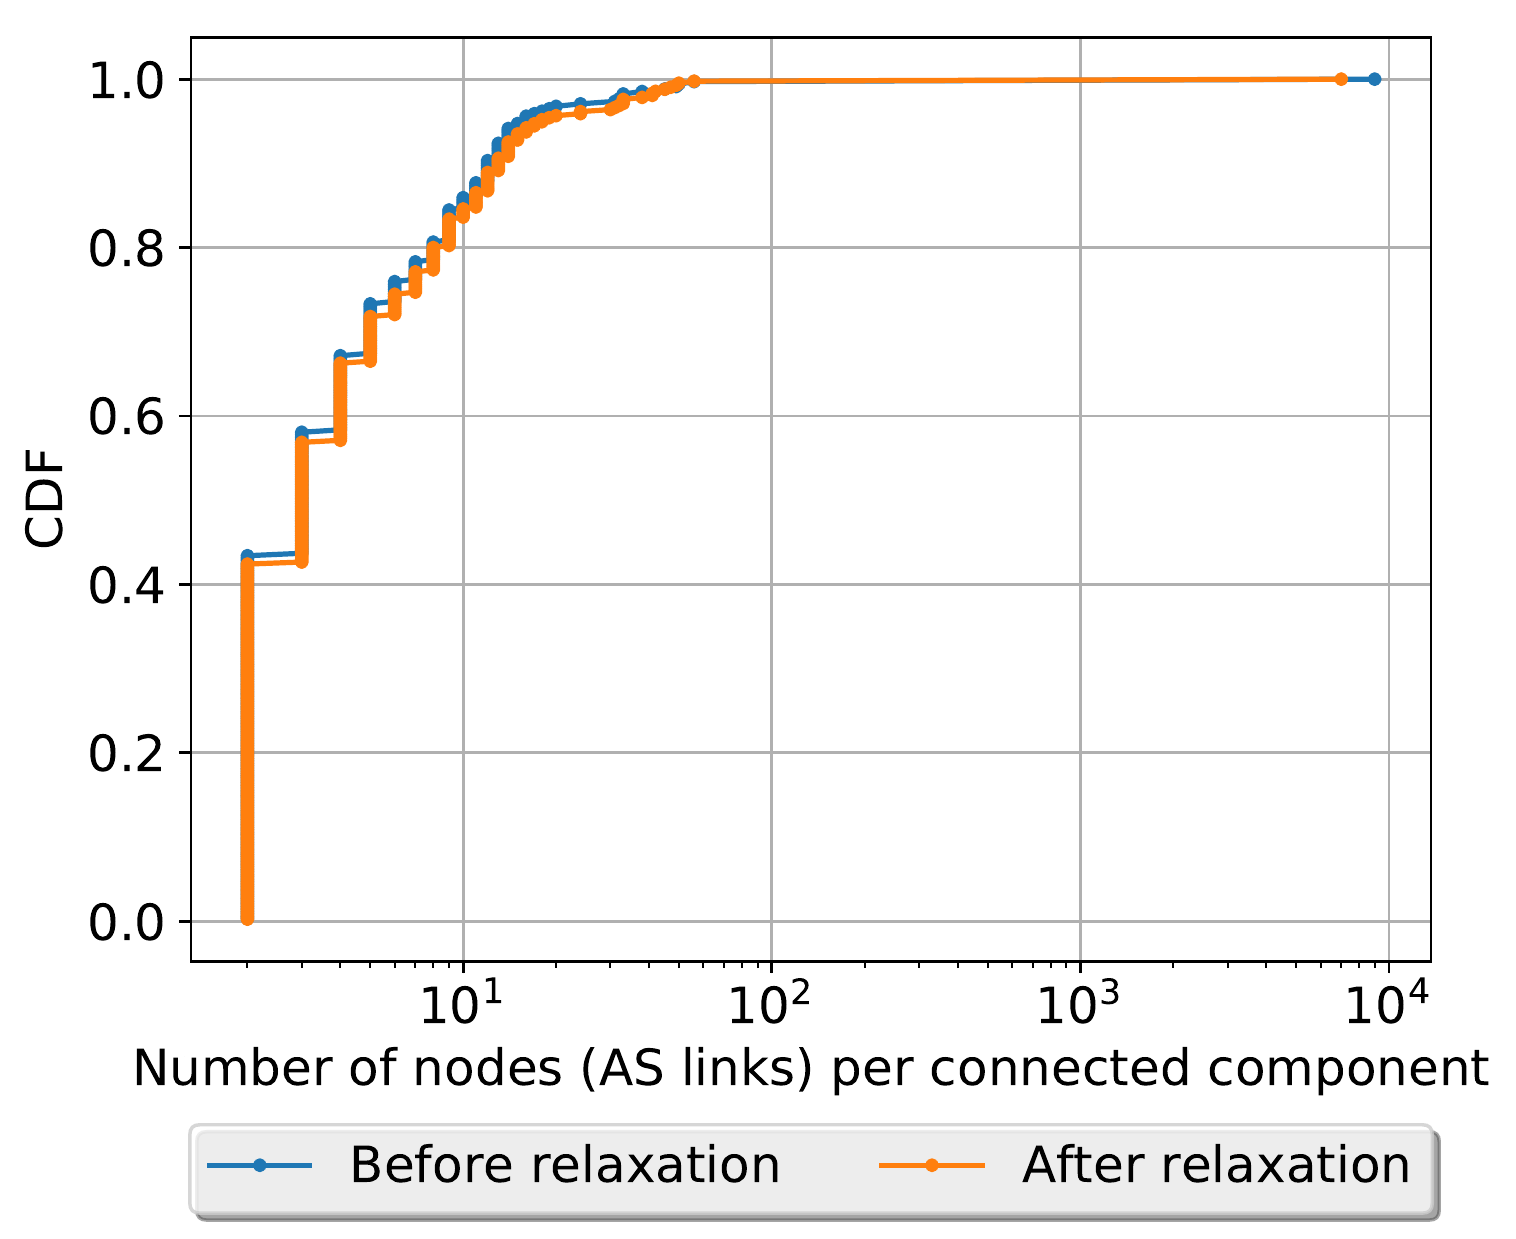}
	\caption{Size distribution of non-trivial connected components. The relaxation step removes a few nodes from the connected components and preserves as much interdependence between the AS links as possible.}
	\label{fig:cc-cdf}
\end{figure}

\subsection{Justification for the Selected Principles}
In this section we provide justification for the two principles used by PARI.

Table~\ref{tab:compare-algo} and~\ref{tab:compare-algo-con} give a comparison of AS inference algorithms. All algorithms rely on the valley-free assumption, except for ASRANK. ASRANK drops it because the assumption is not always valid. Specifically, a study~\cite{qiu2007toward} showed that 14 out of 15 Tier-1 ASes were involved in propagating valley paths. But ASRANK still relies on observations used to derive the valley-free property or assumptions leading to inference results with no valleys. As shown in Table~\ref{tab:compare-algo-con}, ASRANK assumes that a provider announces customer routes to its providers and it forbids adjacent links to be p2p. It means all algorithms are based on the valley-free or other compatible assumptions, which provides the justification for PARI to use it as one of the two principles.

In addition to the valley-free assumption, the inference algorithms develop their own complementary assumptions or rules. But none of them are commonly shared by all algorithms. We believe they are not fundamental to the inference of AS relationships. However, both UCLA and ASRANK make the assumption that a set of large transit providers, connected by p2p links, form a clique at the top of the AS topology. PARI adopts it as another principle because it has been validated by empirical results~\cite{luckie2013relationships}. Since the objective of the principle-based inference step is to infer relationships with high certainty, PARI discards the other assumptions.

\begin{table*}[!htb]
	\centering
	\caption{A comparison of AS relationship inference algorithms}
	\label{tab:compare-algo}
	\begin{tabular}{@{}p{1cm}p{1cm}p{1cm}p{2cm}p{2cm}p{4cm}p{4cm}@{}}
		\toprule
		& Assume valley-free? & Assume Tier-1 clique? & Types of relationships inferred                                                                                                       & Optimization-based? & Strategies to address anomalies                                                                                                                                                                                                                     & Other assumptions and rules                                                                                                                                                                                                                                                                                                                                                                                                                                                       \\ \midrule
		Gao~\cite{gao2001inferring}        & True                & False                 & p2c, p2p, s2s                                                                                                                         & False               & \begin{tabular}[c]{@{}p{4cm}@{}}Combine observations from multiple paths and derive\\ a single decision based on votes\end{tabular}                                                                                                                      & \begin{tabular}[c]{@{}p{4cm}@{}}1. The provider and customer roles are decided by\\ the difference in node degrees. The link is inferred as s2s or p2p if the node\\ degrees are close.\\ 2. The ratio of node degrees of adjacent ASes is\\ compared against the same constant for all links.\end{tabular}                                                                                                                                                                            \\
		Xiao + Gao~\cite{xia2004evaluation} & True                & False                 & p2c, p2p, s2s                                                                                                                         & False               & \begin{tabular}[c]{@{}p{4cm}@{}}Introduce a preprocessing step to filter out\\ non-valley-free paths. Remove infrequent AS paths from the routing tables to reduce\\ the impact of BGP misconfigurations on the accuracy of the inferences.\end{tabular} & \begin{tabular}[c]{@{}p{4cm}@{}}Leverage partial ground-truth obtained from\\ external sources.\end{tabular}                                                                                                                                                                                                                                                                                                                                                                           \\
		MVP~\cite{subramanian2002characterizing}        & True                & False                 & p2c, p2p                                                                                                                              & False               & N/A                                                                                                                                                                                                                                                 & \begin{tabular}[c]{@{}p{4cm}@{}}1. Given the directed graph constructed from the AS\\ paths received by a single vantage point (root node), the leaf nodes are likely\\ to be the customers of their parent nodes.\\ 2. The root nodes receive the highest rank and the\\ leaf nodes the lowest. A node with higher rank is more likely to be the\\ provider. Ranks given by multiple vantage points are combined to overcome the\\ limitation of a single vantage point.\end{tabular} \\
		DPP~\cite{di2003computing}        & True                & False                 & \begin{tabular}[c]{@{}p{2cm}@{}}p2c (p2p links can be derived from a p2c-only solution,\\ but no specific algorithm is given)\end{tabular} & True                & \begin{tabular}[c]{@{}p{4cm}@{}}To address the problem of valley paths, it\\ applies a heuristic to identify a large subset of paths that admit valley-free\\ assignment.\end{tabular}                                                                   & N/A                                                                                                                                                                                                                                                                                                                                                                                                                                                                               \\
		ARIV~\cite{dimitropoulos2007relationships}       & True                & False                 & p2c, p2p                                                                                                                              & True                & \begin{tabular}[c]{@{}p{4cm}@{}}Collect multiple datasets over different periods\\ and remove transient paths.\end{tabular}                                                                                                                               & \begin{tabular}[c]{@{}p{4cm}@{}}1. The orientation of p2c relationships follows relative difference in node degrees and small difference indicates p2p relationships.\\ 2. The degree of small ASes are underestimated.\end{tabular}                                                                                                                                                                                                                                                   \\
		UCLA \cite{oliveira2010completeness}       & True                & True                  & p2c, p2p                                                                                                                              & False               & N/A                                                                                                                                                                                                                                                 & \begin{tabular}[c]{@{}p{4cm}@{}}1. The set of Tier-1 ASes are given.\\ 2. Monitors located in Tier-1 should be able to\\ reveal all p2c relationships over time.\end{tabular}                                                                                                                                                                                                                                                                                                          \\
%		ASRANK~\cite{luckie2013relationships}     & False               & True                  & p2c, p2p                                                                                                                              & False               & \todo{too long  to fit in page}                                                                                                                                                                                                                                              & \todo{too long  to fit in page}                                                                                                                                                                                                                                                                                                                                                                                                                                                                     \\
		\bottomrule
	\end{tabular}
\end{table*}

\begin{table*}[!htb]
	\centering
	\caption{A comparison of AS relationship inference algorithms (Cont.)}
	\label{tab:compare-algo-con}
	\begin{tabular}{@{}p{1cm}p{1cm}p{1cm}p{2cm}p{2cm}p{4cm}p{4cm}@{}}
		\toprule
		& Assume valley-free? & Assume Tier-1 clique? & Types of relationships inferred                                                                                                       & Optimization-based? & Strategies to address anomalies                                                                                                                                                                                                                     & Other assumptions and rules                                                                                                                                                                                                                                                                                                                                                                                                                                                       \\ \midrule
		ASRANK \cite{luckie2013relationships} & False               & True                  & p2c, p2p                        & False               & \begin{tabular}[c]{@{}p{4cm}@{}}1. Filter out poisoned paths.\\ 2. Filter out paths with unassigned AS numbers.\\ 3. Remove ASes used for IXP route servers.\end{tabular} & \begin{tabular}[c]{@{}p{4cm}@{}}1. The largest transit providers, by transit degree, form a clique of p2p links.\\ 2. A provider announces customer routes to its providers.\\ 3. Cycles of p2c links are not allowed.\\ 4. p2c relationships typically follow degree gradient to prevent cycles.\\ 5. Vantage points reporting routes to less than 2.5\% of ASes are not announcing provider routes.\\ 6. Adjacent p2p links are not allowed.\end{tabular} \\ \bottomrule
	\end{tabular}
\end{table*}
